# Supplementary material for: CHANG-ES XXVI: Insights into cosmic-ray transport from radio halos in edge-on galaxies
Source: arXiv:2210.07709 source file (2022-10-14)
Supplement: Supplementary file 3 [file spinnaker_appendix.tex]

%n891
\begin{figure*}
\centering
\begin{subfigure}{0.49\linewidth}
\centering
\includegraphics[width=1\linewidth]{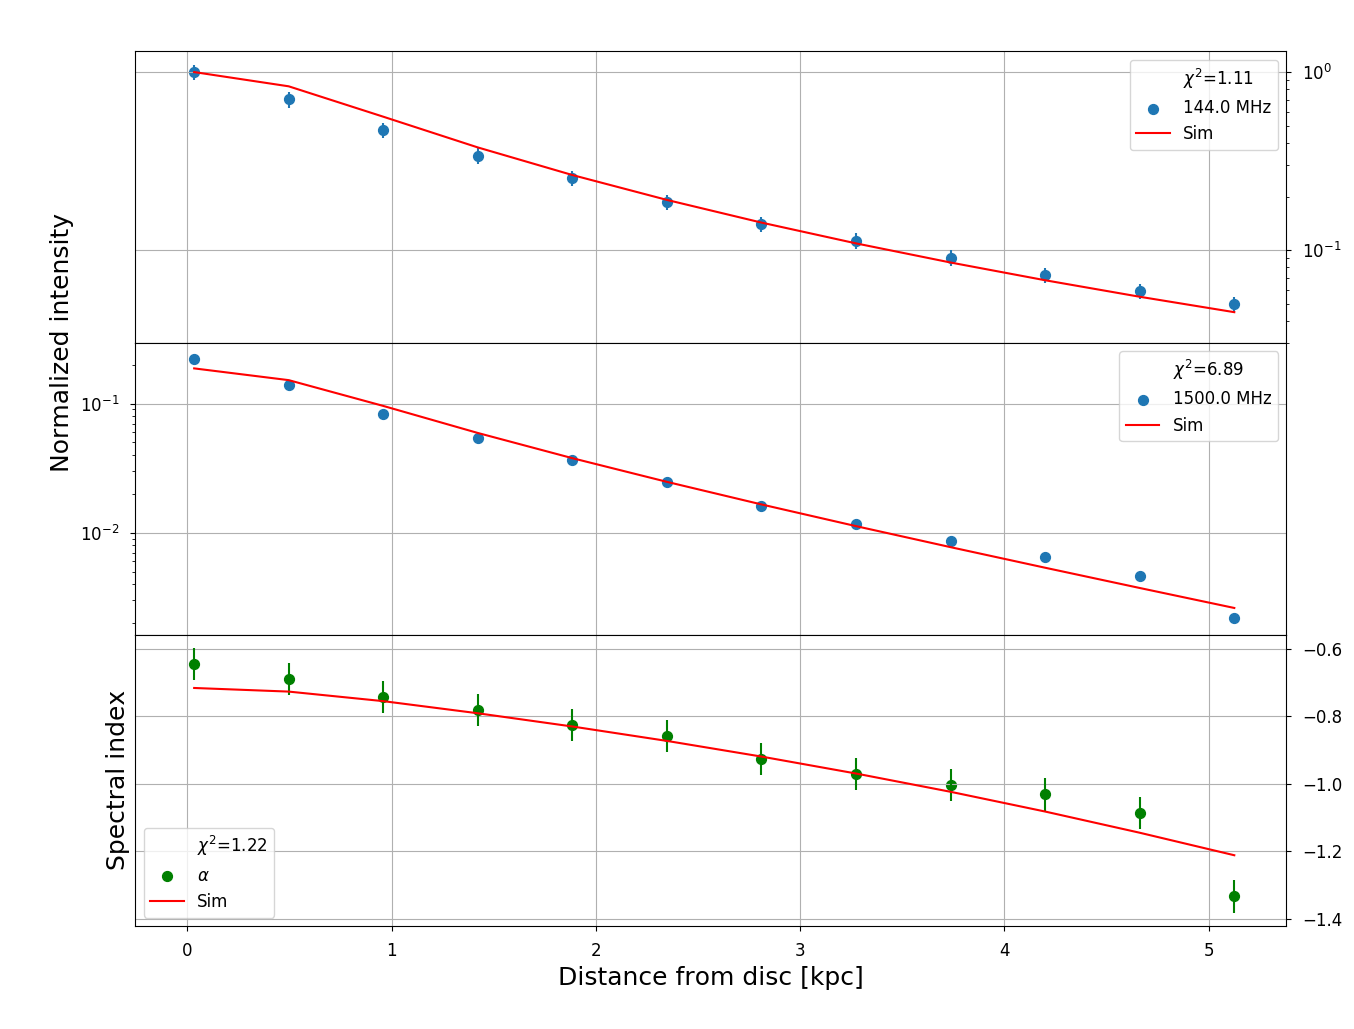}
\end{subfigure}
\hfill
\begin{subfigure}{0.49\linewidth}
\centering
\includegraphics[width=1\linewidth]{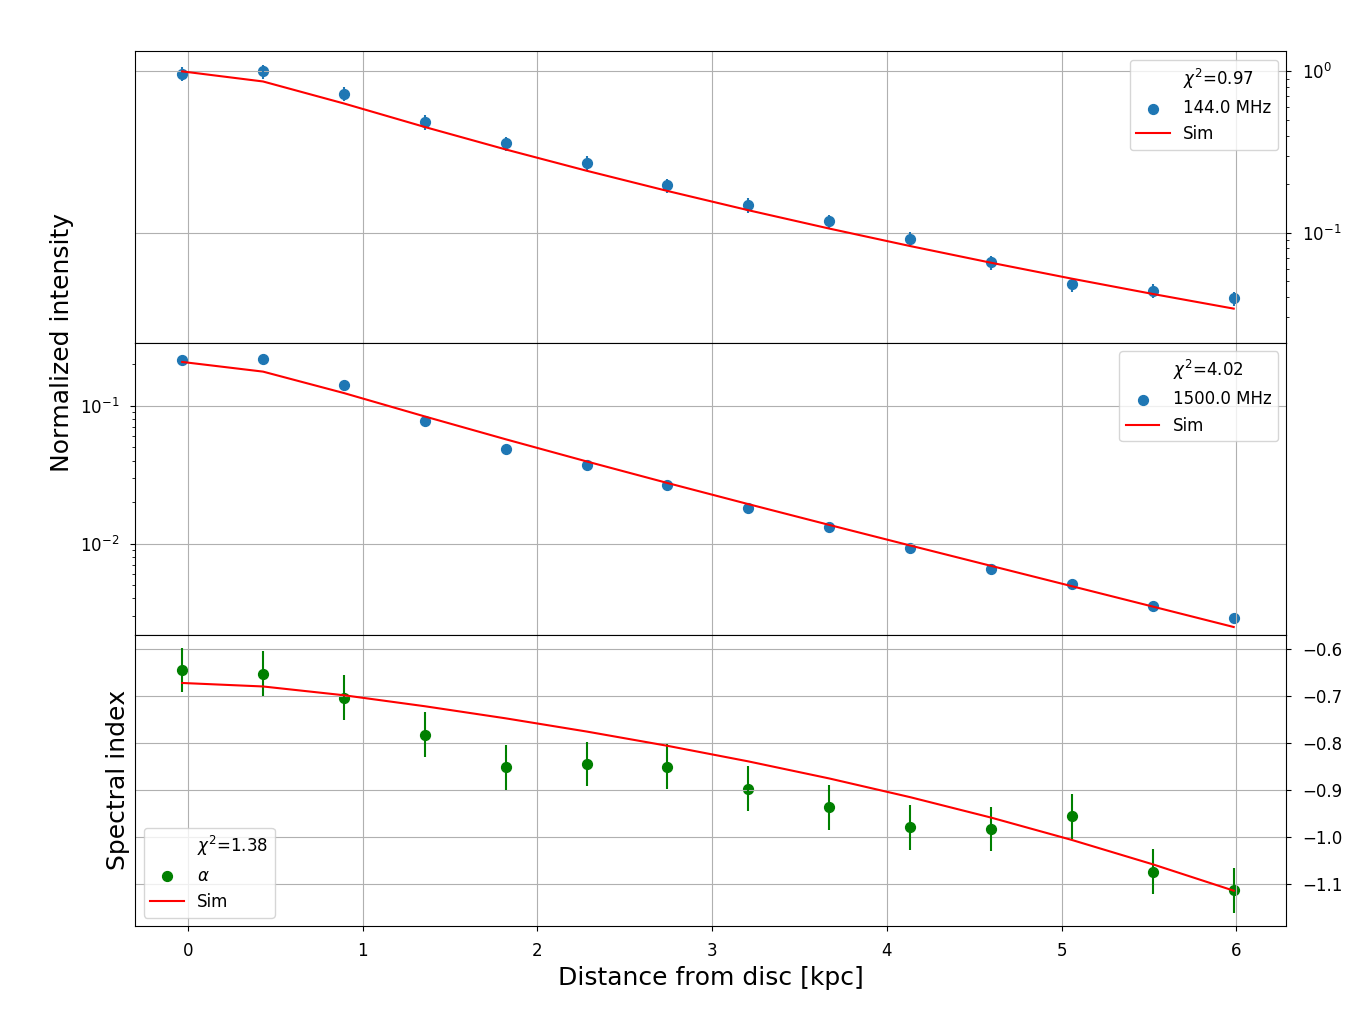}
\end{subfigure}
\\
\begin{subfigure}{0.49\linewidth}
\centering
\includegraphics[width=1\linewidth]{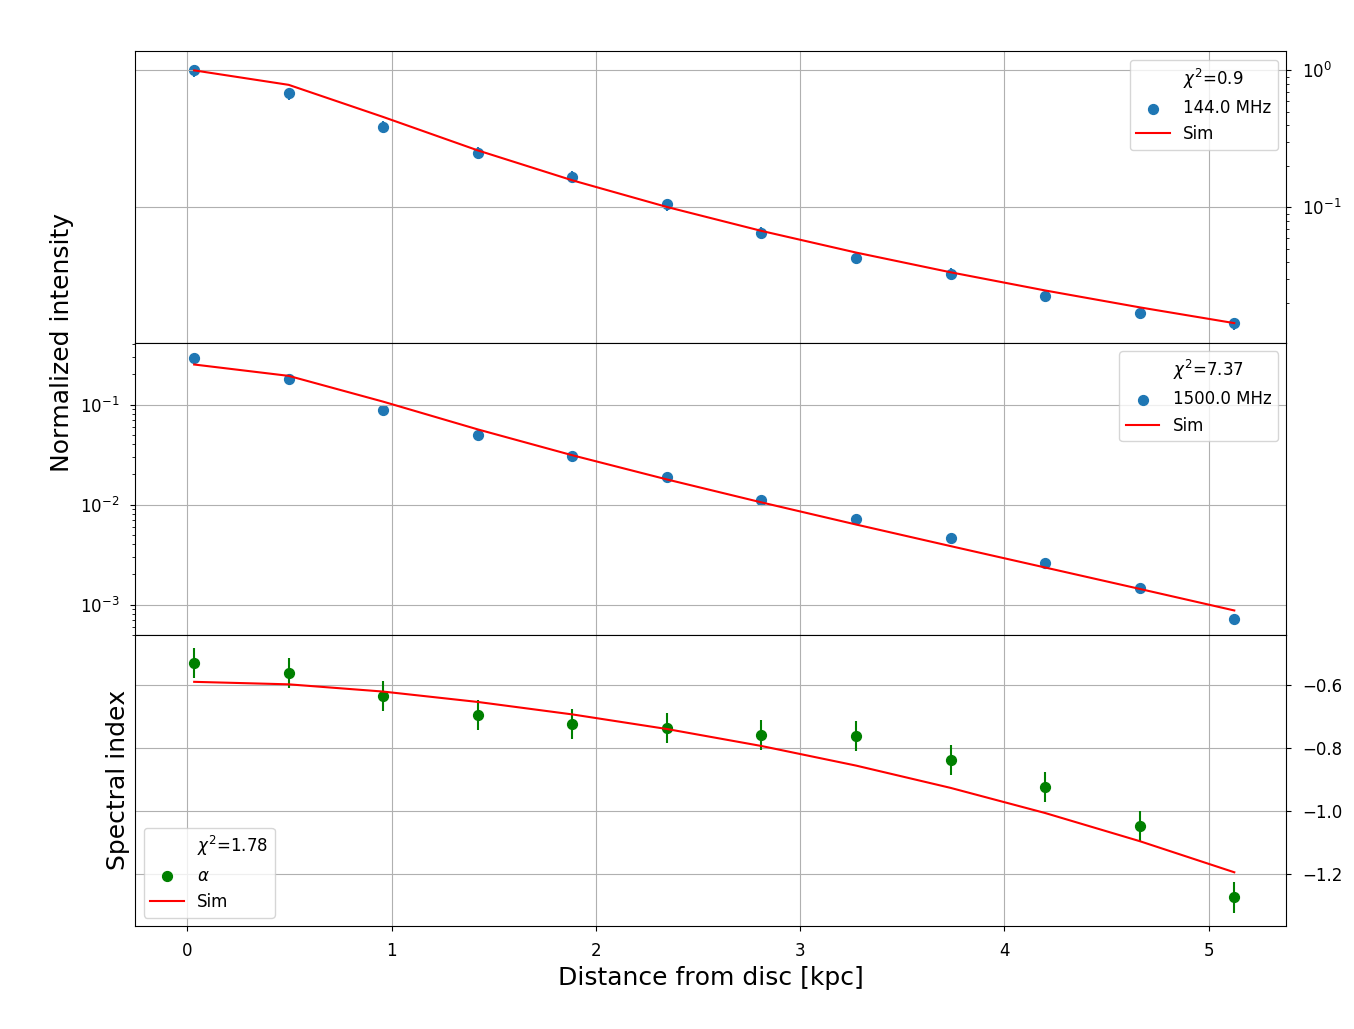}
\end{subfigure}
\hfill
\begin{subfigure}{0.49\linewidth}
\centering
\includegraphics[width=1\linewidth]{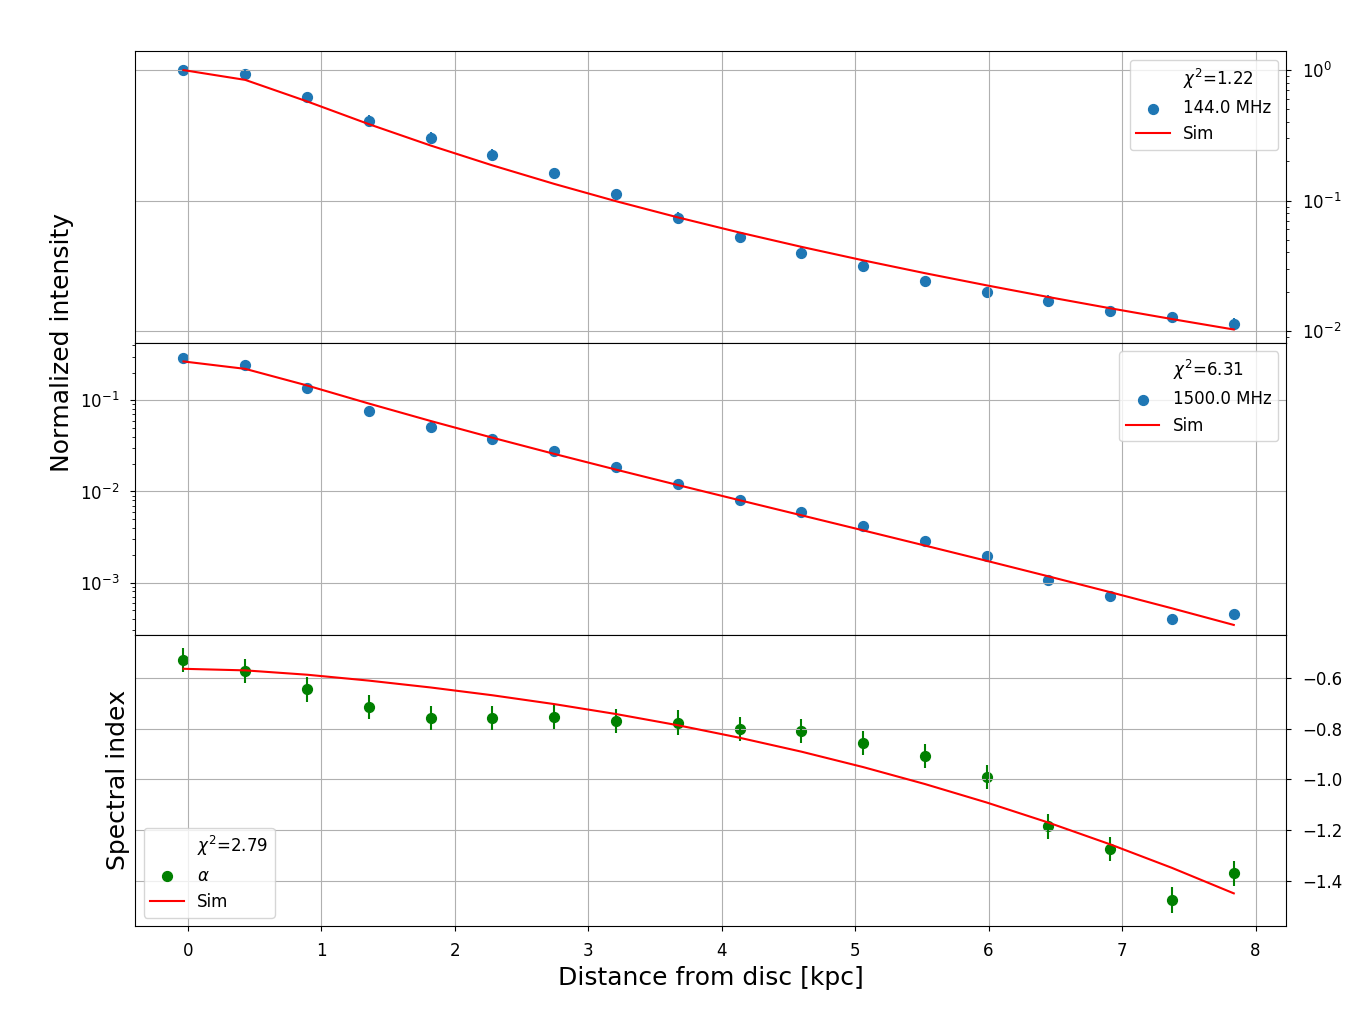}
\end{subfigure}
\\
\begin{subfigure}{0.49\linewidth}
\centering
\includegraphics[width=1\linewidth]{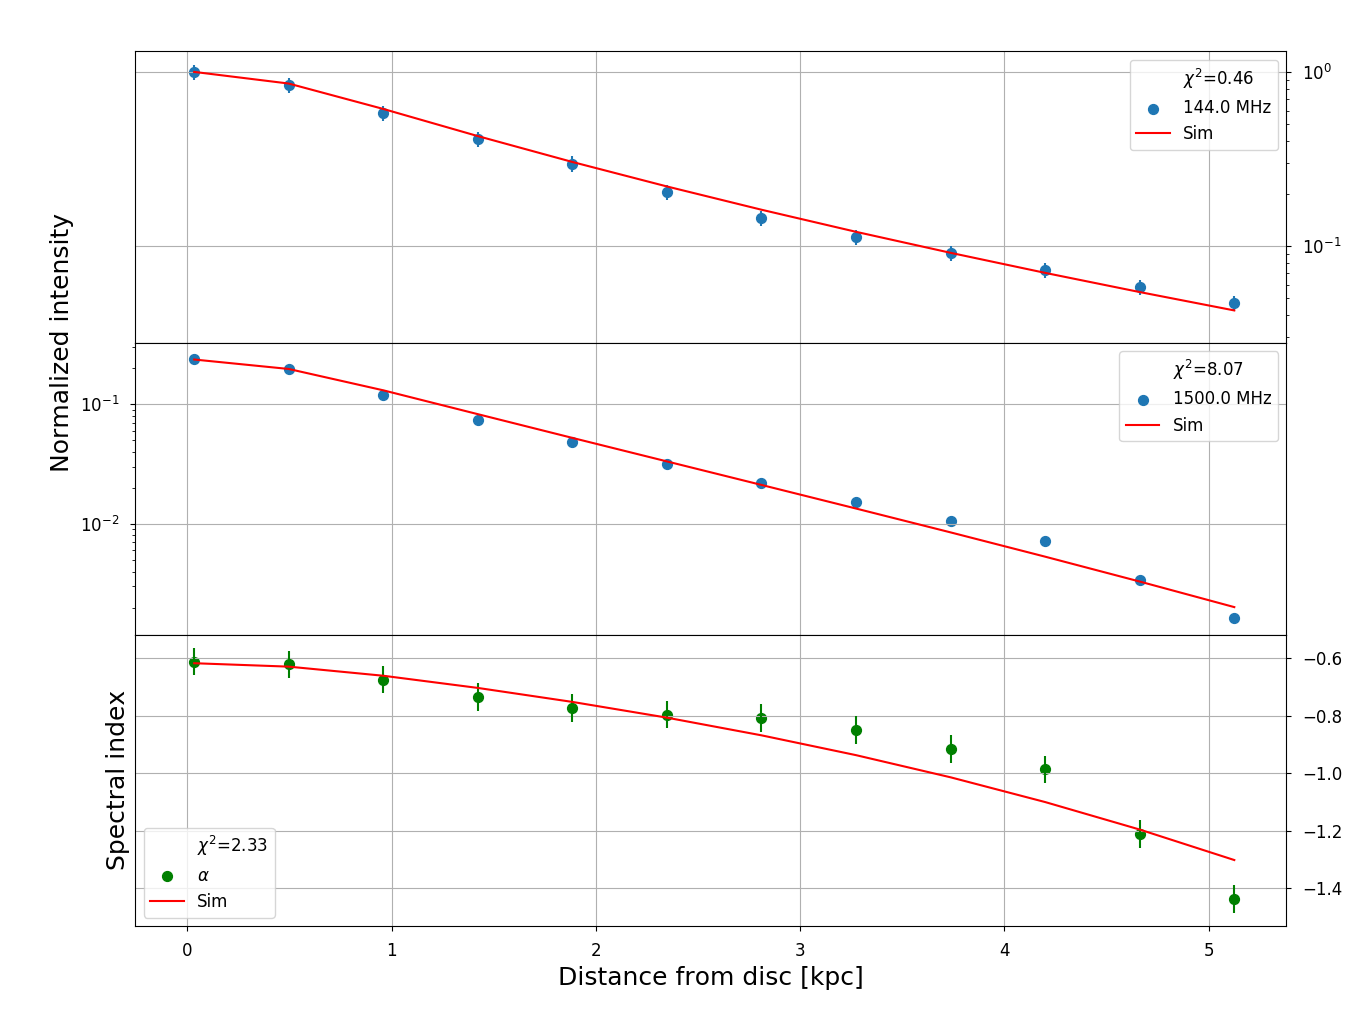}
\end{subfigure}
\hfill
\begin{subfigure}{0.49\linewidth}
\centering
\includegraphics[width=1\linewidth]{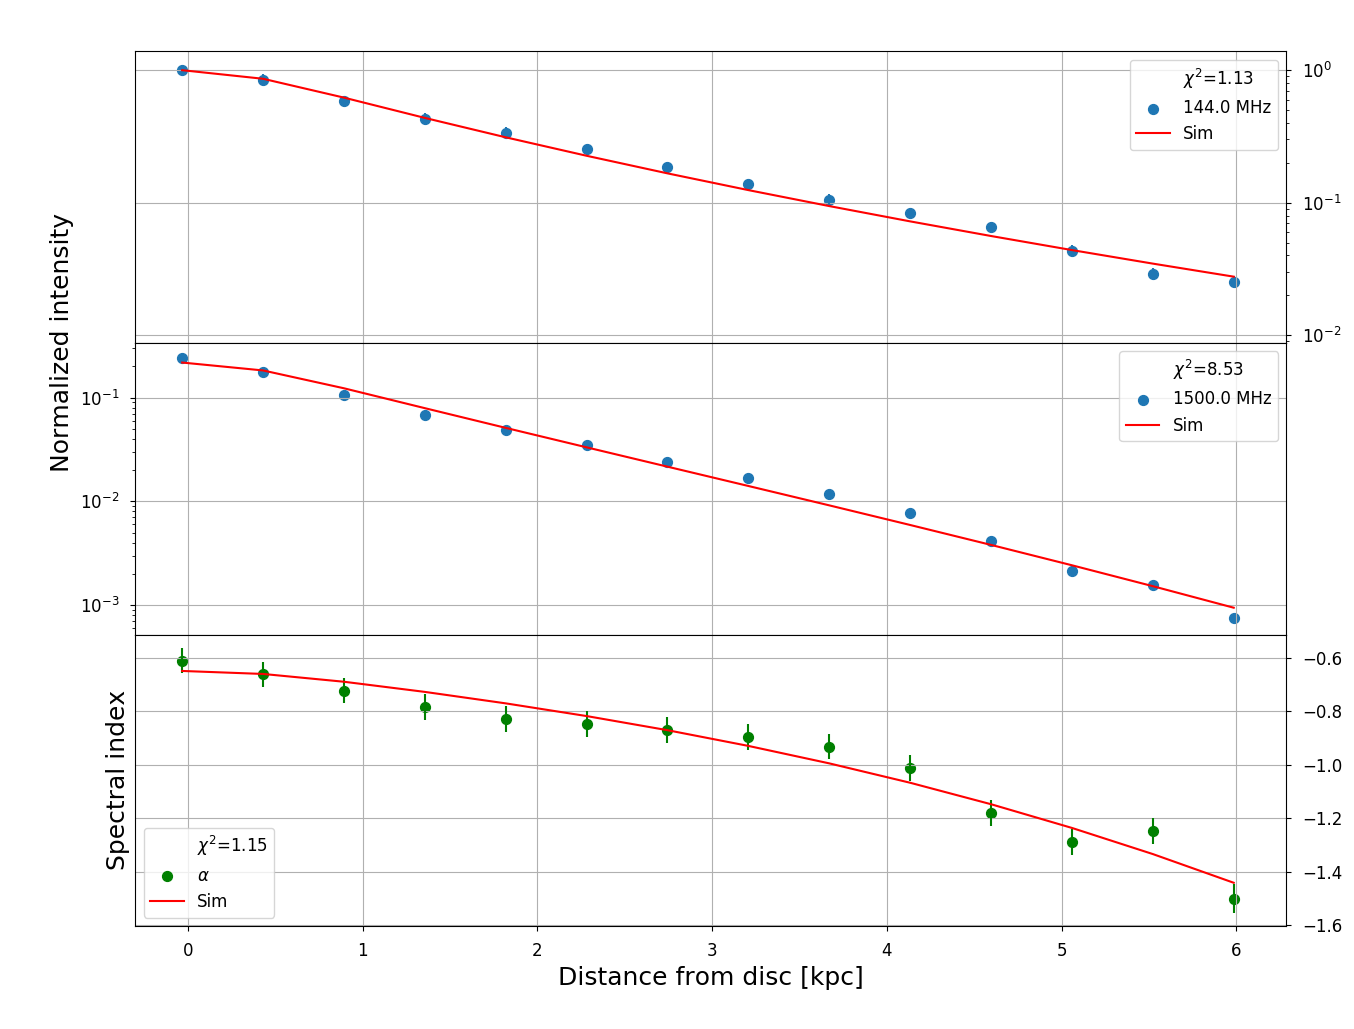}
\end{subfigure}
\caption{\texttt{SPINNAKER} profiles of NGC~891 (all advection). Strips are presented as follows: top left: LR, top right: UR, middle left: LM, middle right: UM, bottom left: LL, and bottom right: UL.}
\end{figure*}
%n3432
\begin{figure*}
\centering
\begin{subfigure}{0.49\linewidth}
\centering
\includegraphics[width=1\linewidth]{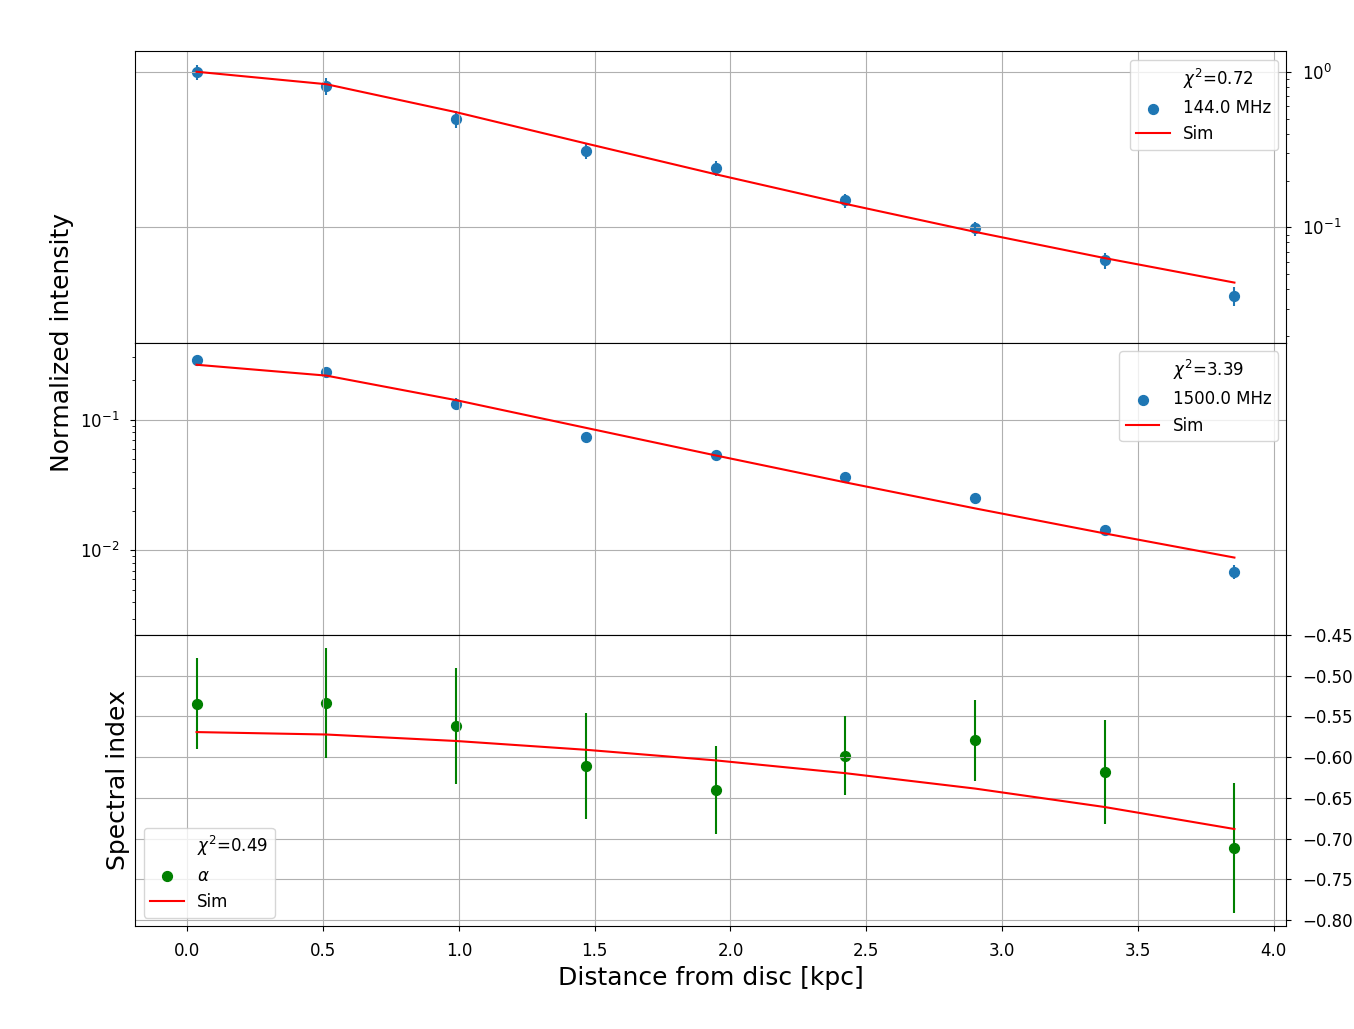}
\end{subfigure}
\hfill
\begin{subfigure}{0.49\linewidth}
\centering
\includegraphics[width=1\linewidth]{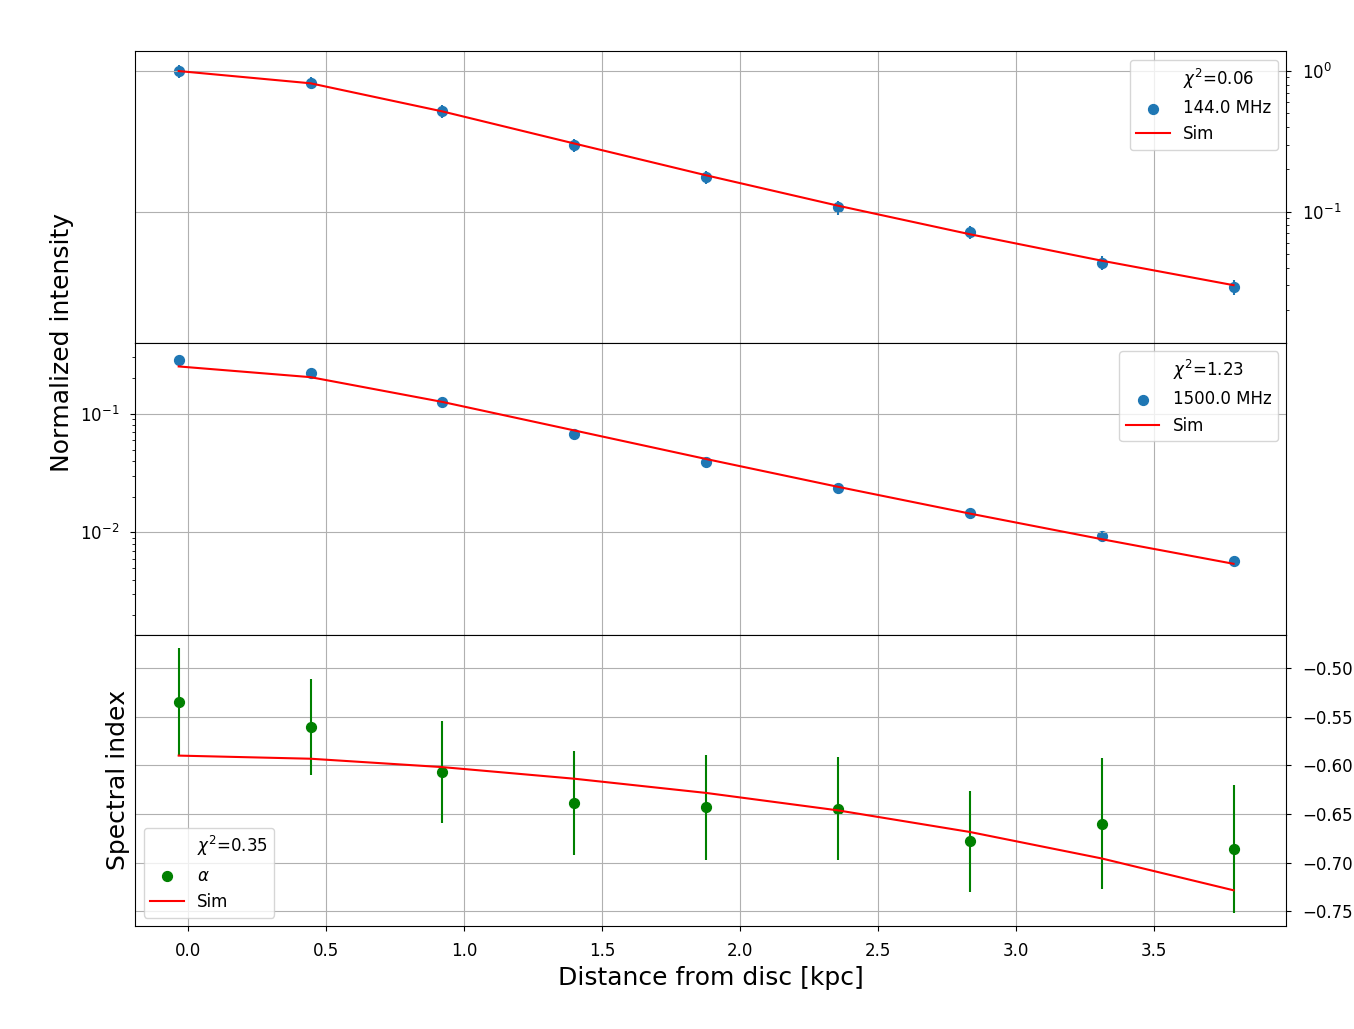}
\end{subfigure}
\caption{\texttt{SPINNAKER} profiles of NGC~3432 (all advection). Strips are presented as follows: left: LM and right: UM.}
\end{figure*}

%n4013
\begin{figure*}
\centering
\begin{subfigure}{0.49\linewidth}
\centering
\includegraphics[width=1\linewidth]{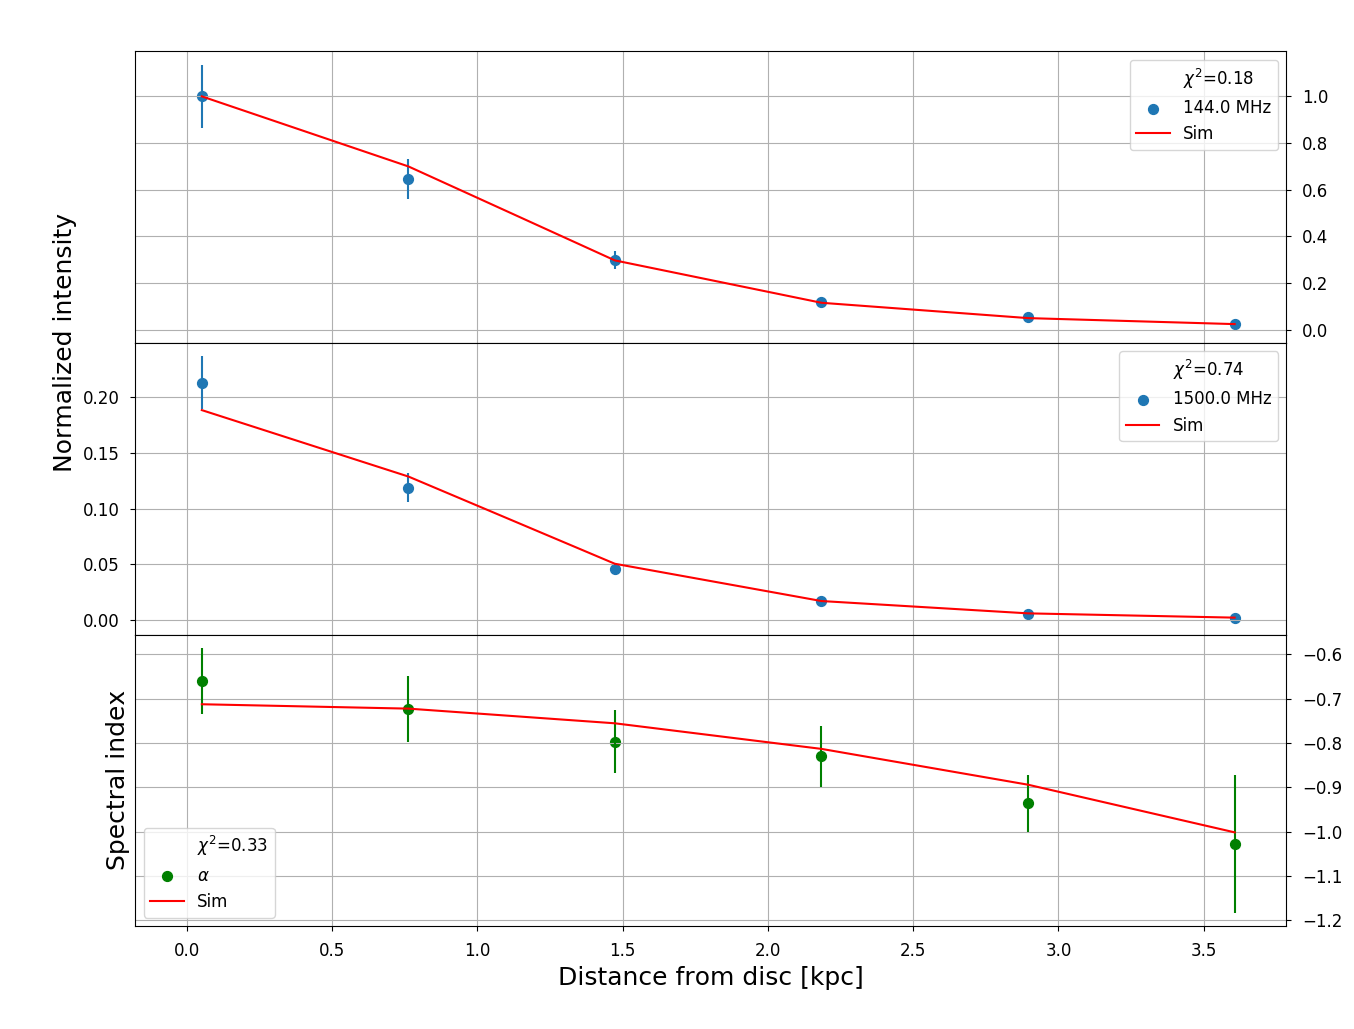}
\end{subfigure}
\hfill
\begin{subfigure}{0.49\linewidth}
\centering
\includegraphics[width=1\linewidth]{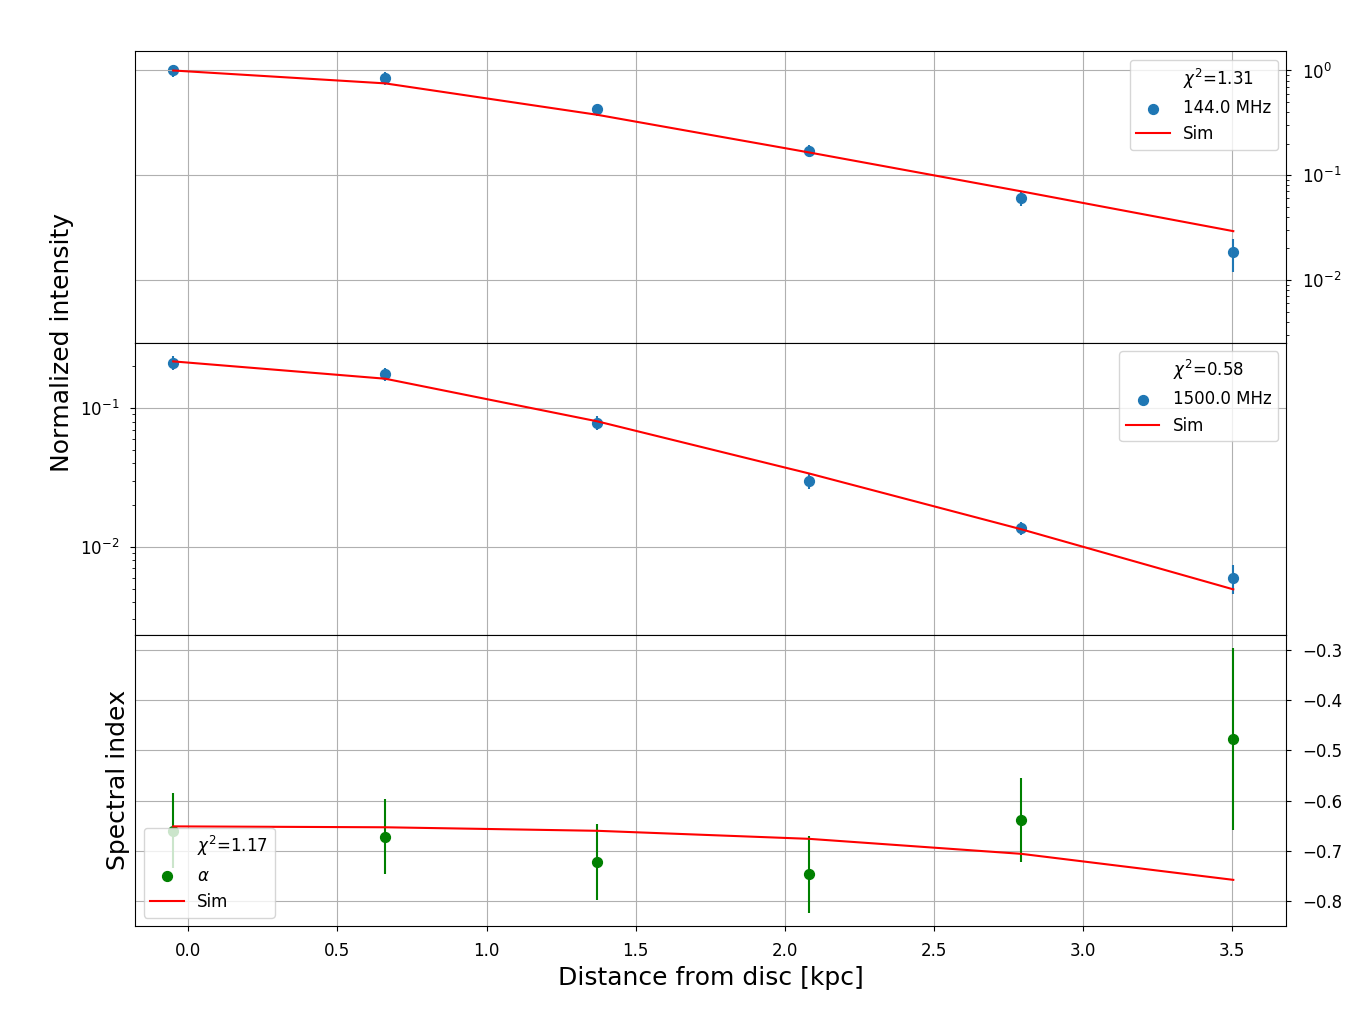}
\end{subfigure}
\\
\begin{subfigure}{0.49\linewidth}
\centering
\includegraphics[width=1\linewidth]{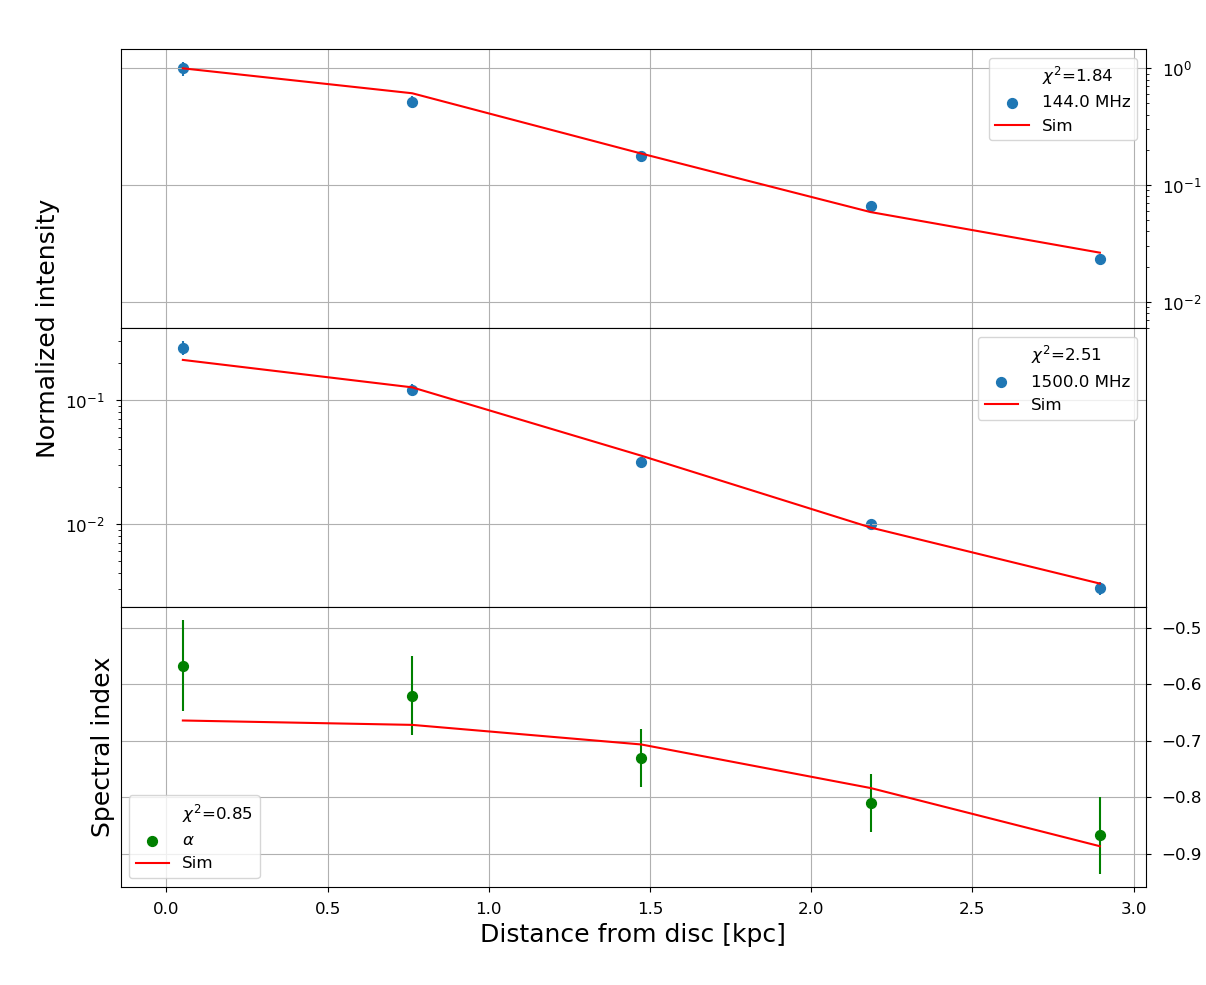}
\end{subfigure}
\hfill
\begin{subfigure}{0.49\linewidth}
\centering
\includegraphics[width=1\linewidth]{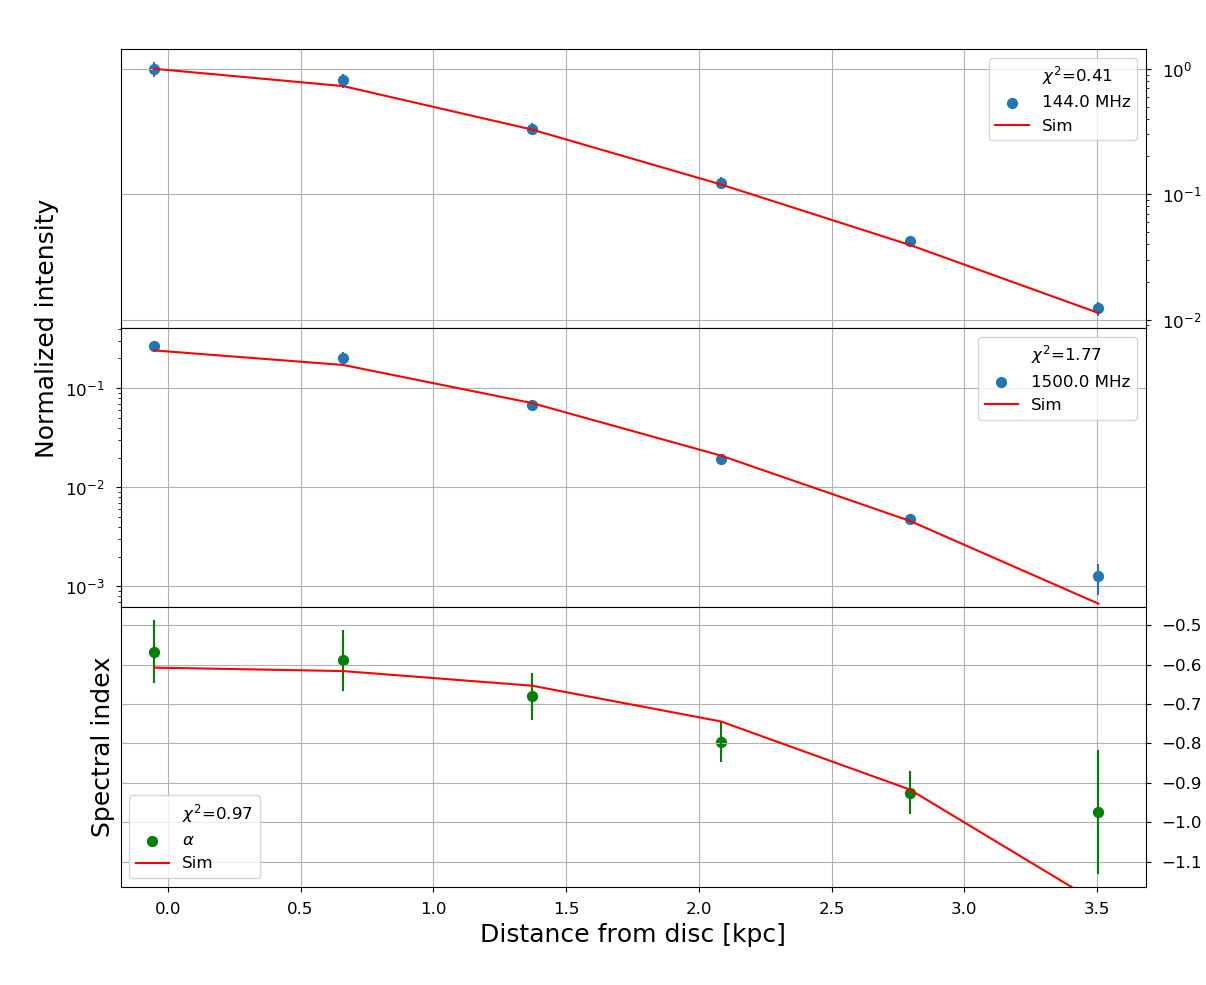}
\end{subfigure}
\\
\begin{subfigure}{0.49\linewidth}
\centering
\includegraphics[width=1\linewidth]{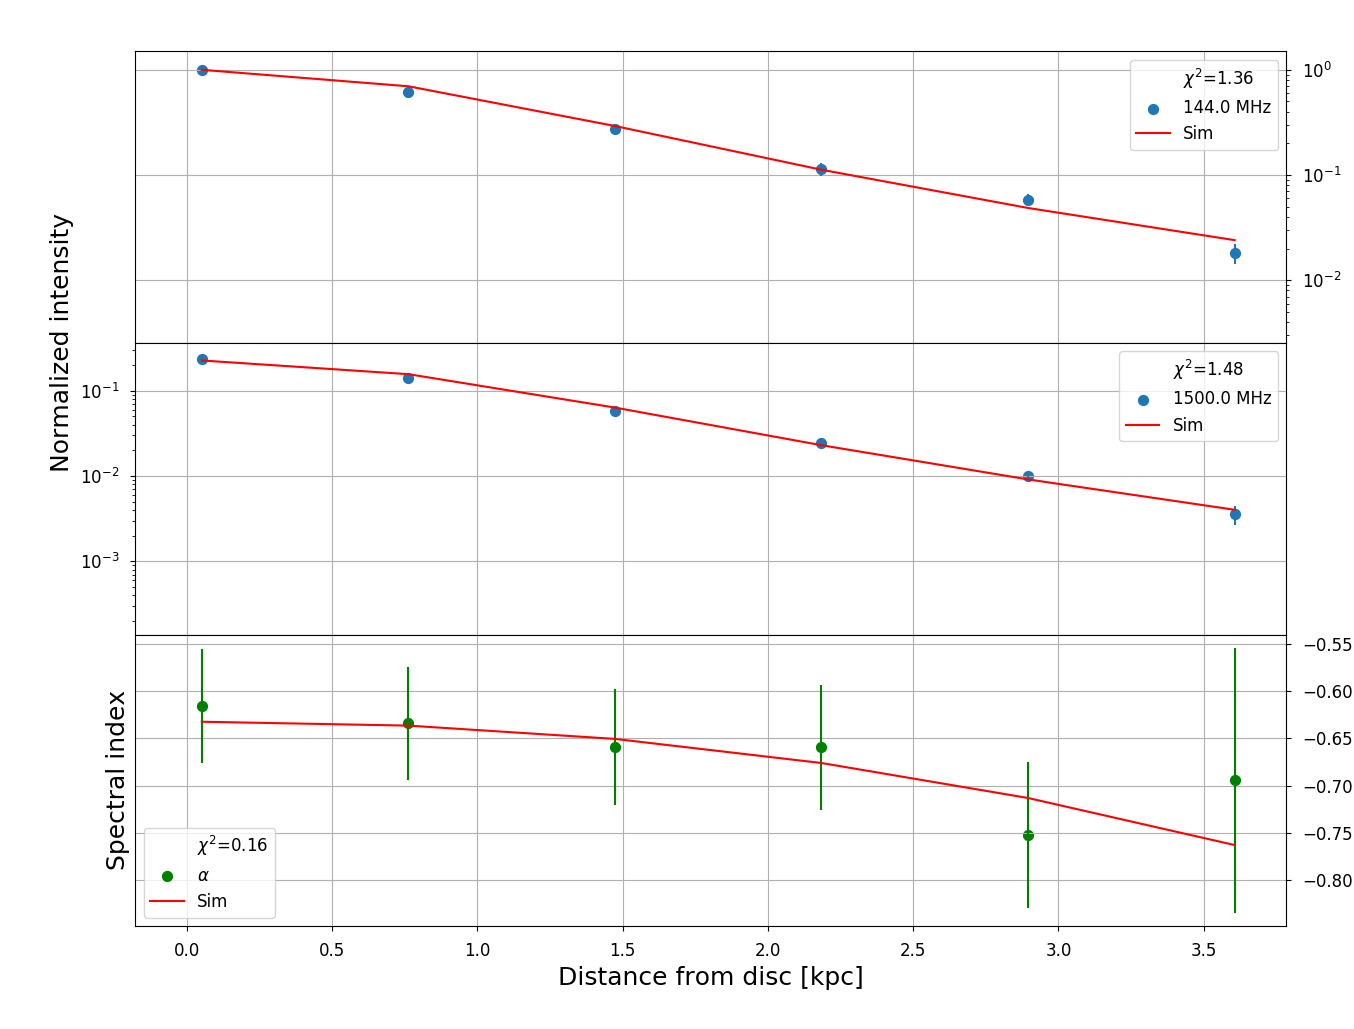}
\end{subfigure}
\hfill
\begin{subfigure}{0.49\linewidth}
\centering
\includegraphics[width=1\linewidth]{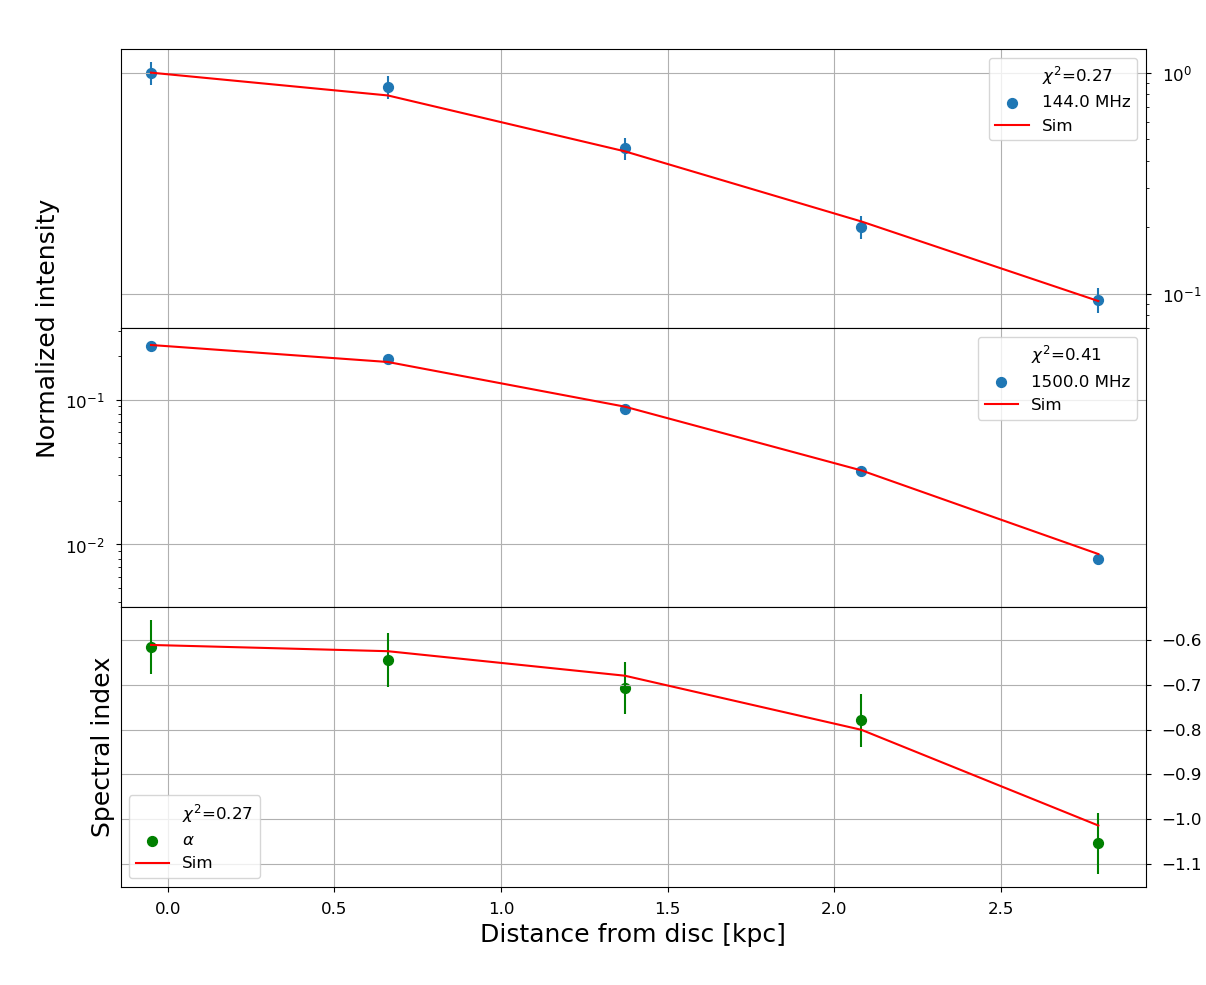}
\end{subfigure}
\caption{\texttt{SPINNAKER} profiles of NGC~4013. Strips are presented as follows: top left: LR (advection), top right: UR (diffusion), middle left: LM (advection), middle right: UM (diffusion), bottom left: LL (advection), and bottom right: UL (diffusion).}
\end{figure*}

%n4157
\begin{figure*}
\centering
\begin{subfigure}{0.49\linewidth}
\centering
\includegraphics[width=1\linewidth]{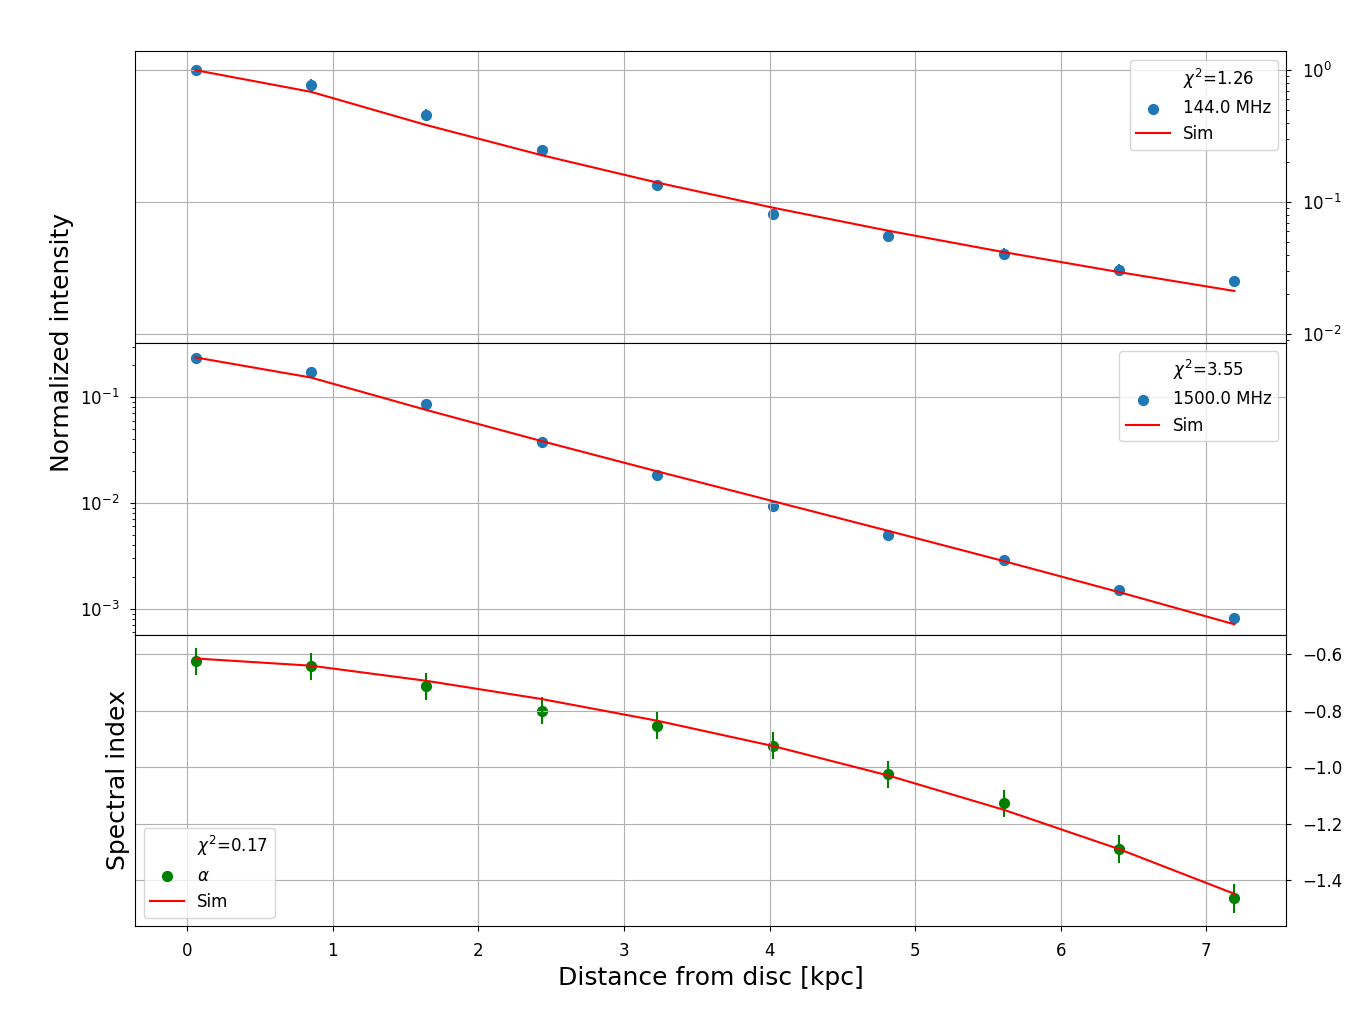}
\end{subfigure}
\hfill
\begin{subfigure}{0.49\linewidth}
\centering
\includegraphics[width=1\linewidth]{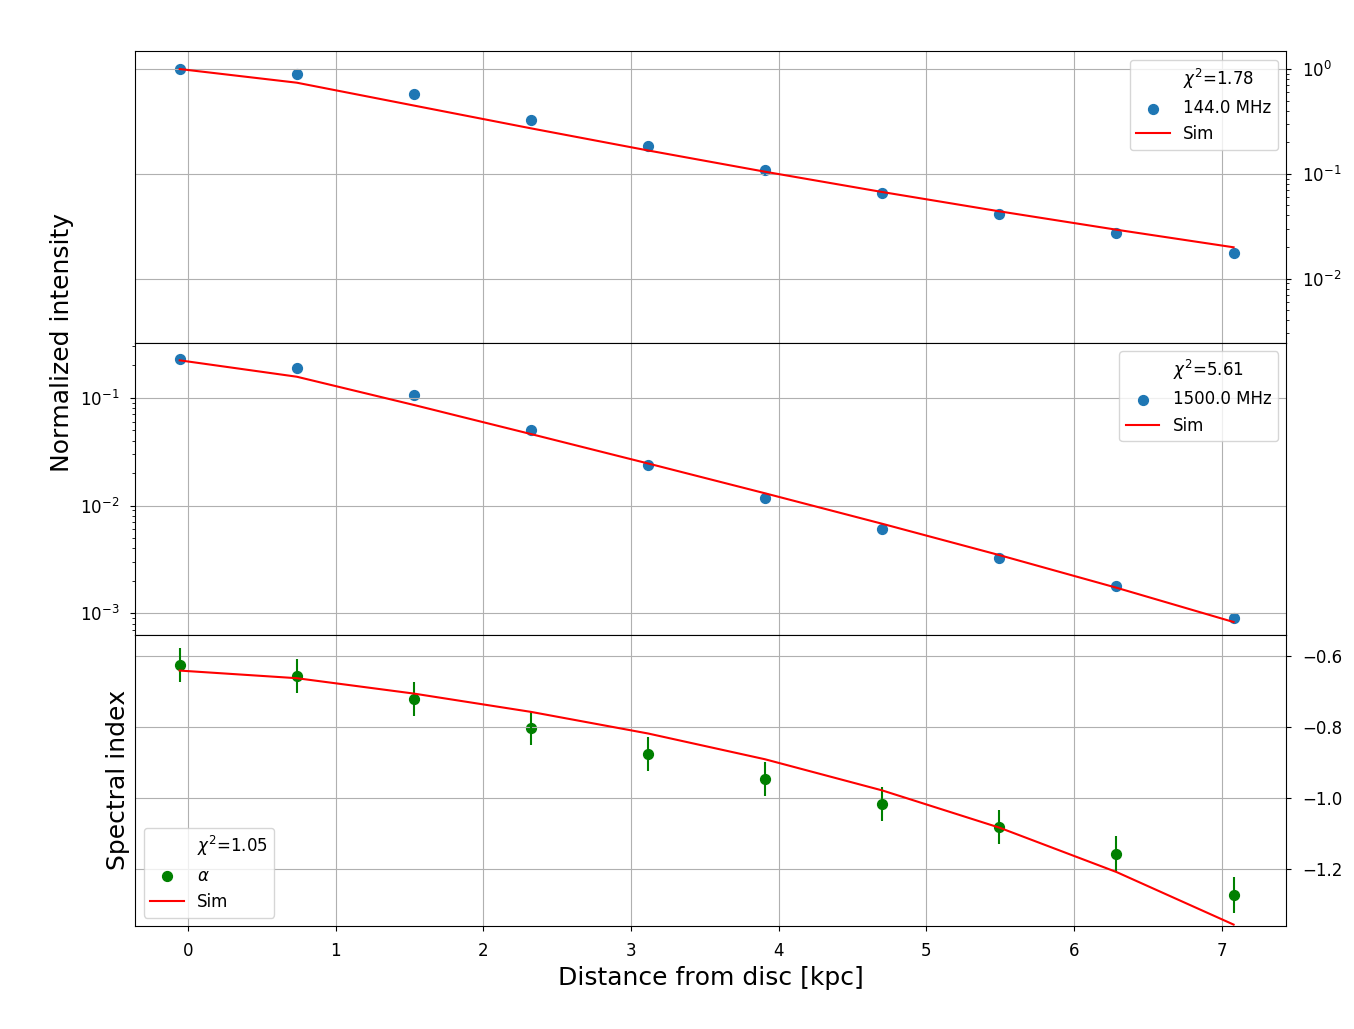}
\end{subfigure}
\\
\begin{subfigure}{0.49\linewidth}
\centering
\includegraphics[width=1\linewidth]{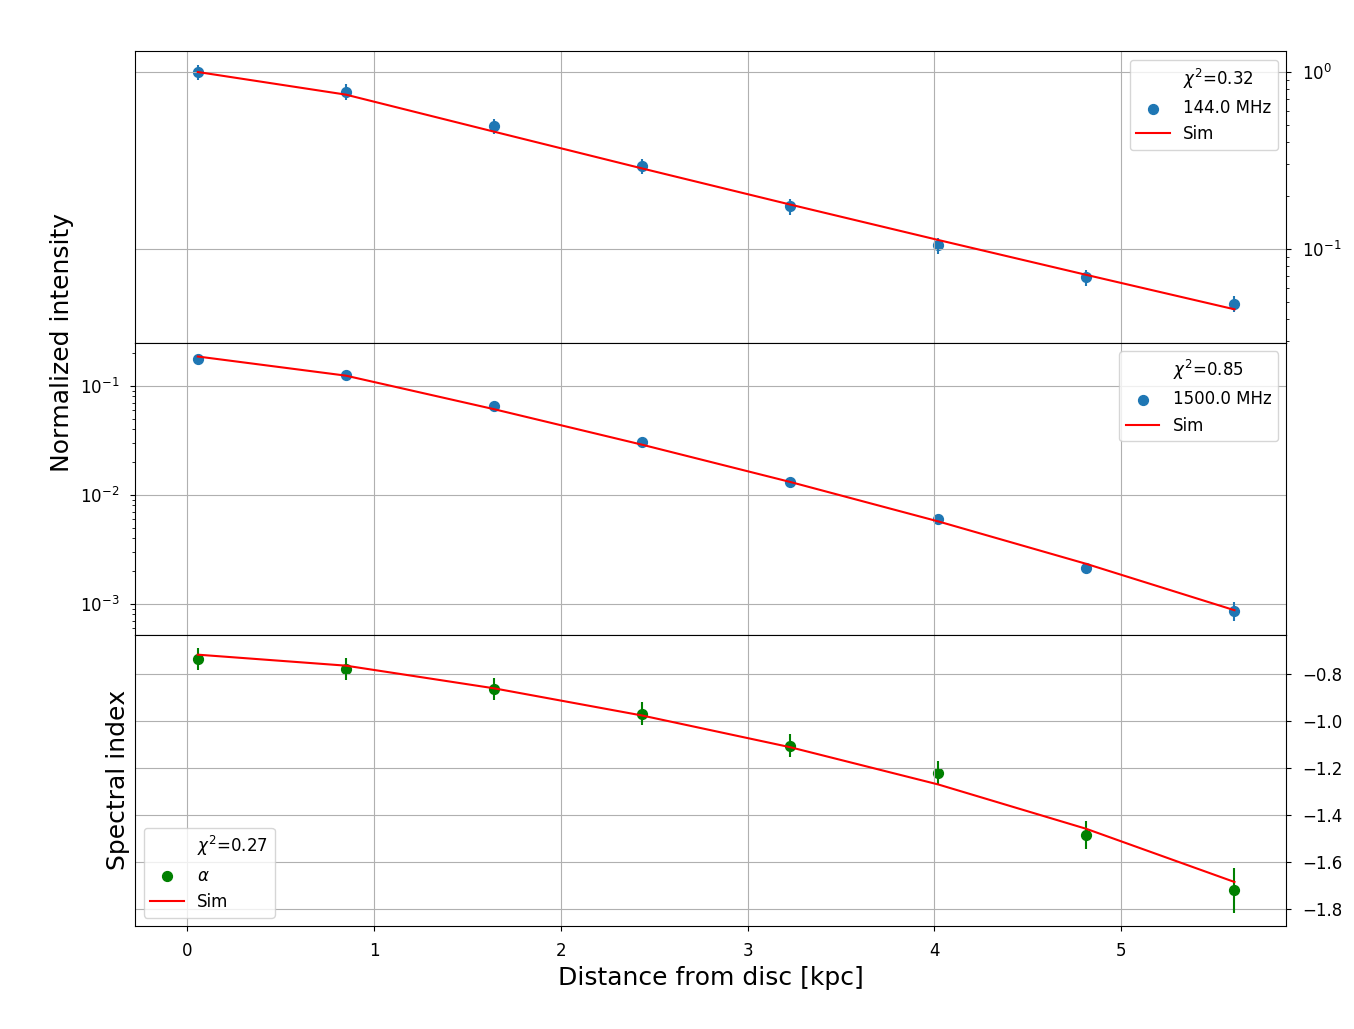}
\end{subfigure}
\hfill
\begin{subfigure}{0.49\linewidth}
\centering
\includegraphics[width=1\linewidth]{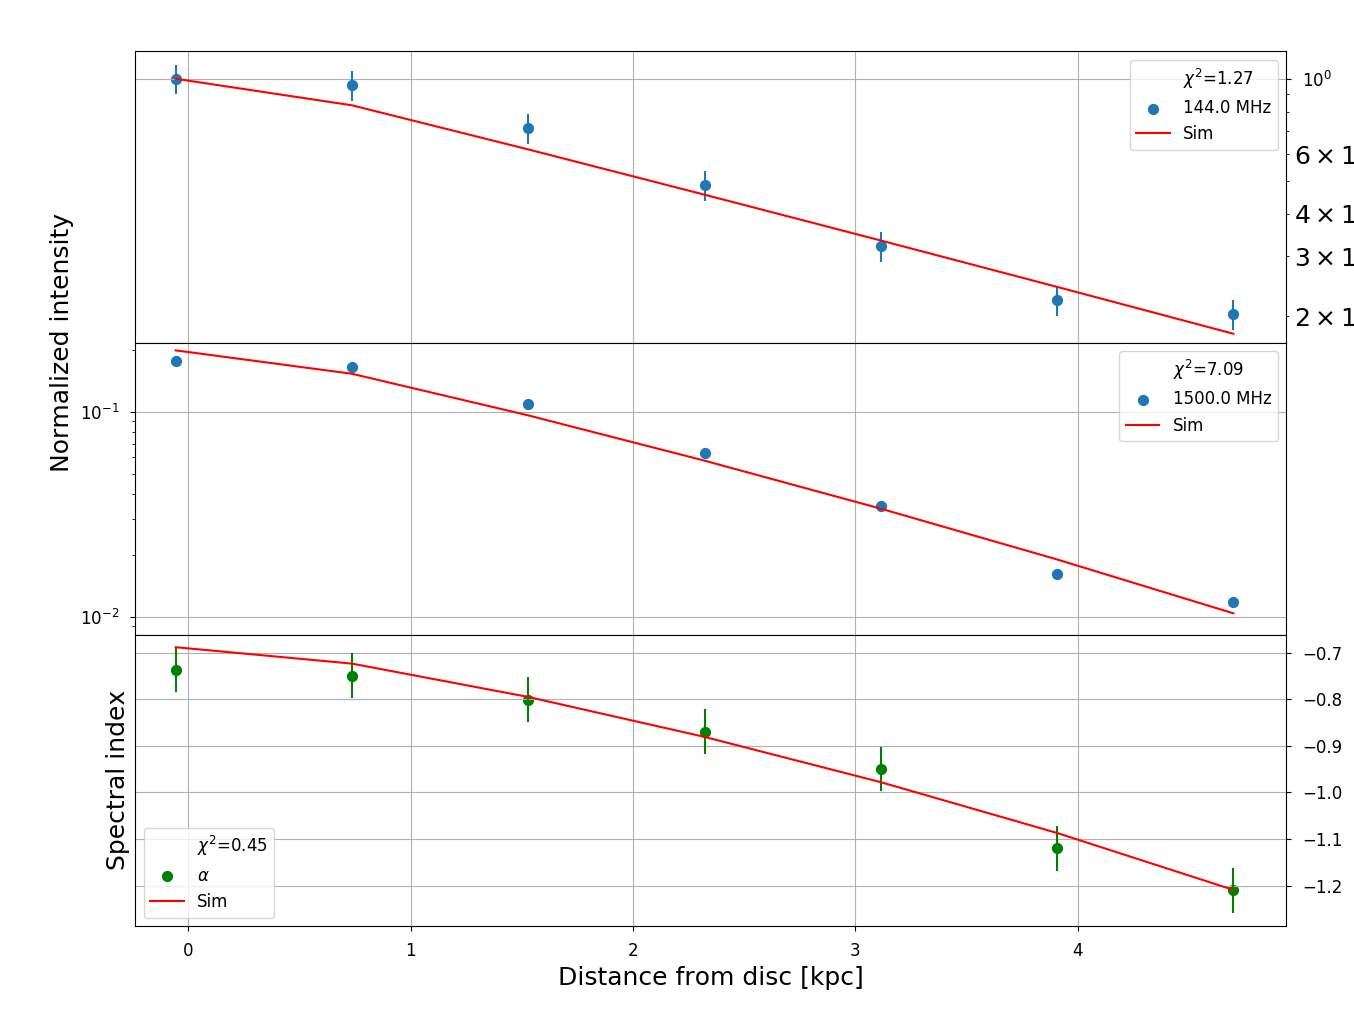}
\end{subfigure}
\caption{\texttt{SPINNAKER} profiles of NGC~4157 (all advection). Stripes are present as follows: top left: LM, top right: UM, bottom left: LL, and bottom right: UL.}
\end{figure*}

%n4631
\begin{figure*}
\centering
\begin{subfigure}{0.49\linewidth}
\centering
\includegraphics[width=1\linewidth]{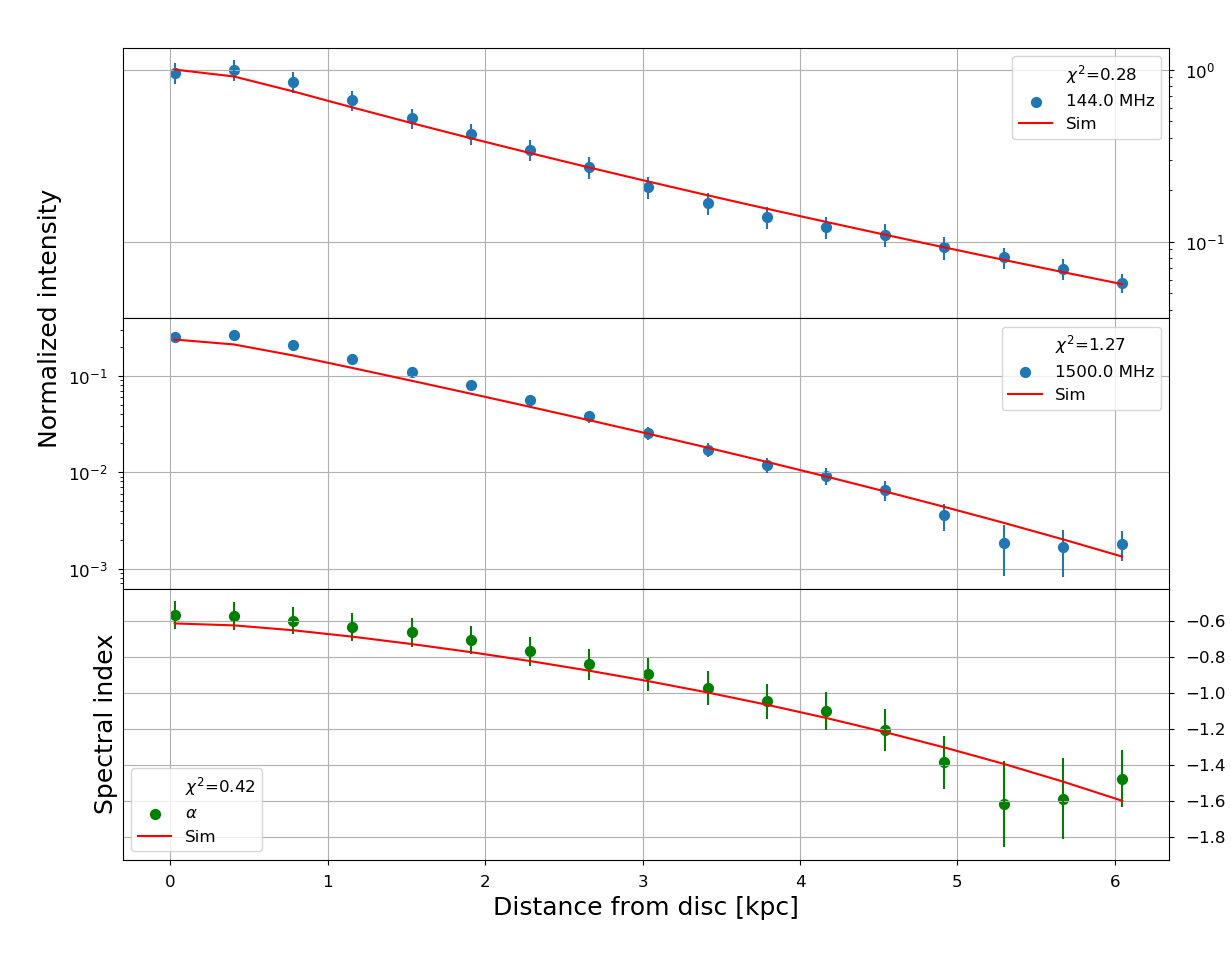}
\end{subfigure}
\hfill
\begin{subfigure}{0.49\linewidth}
\centering
\includegraphics[width=1\linewidth]{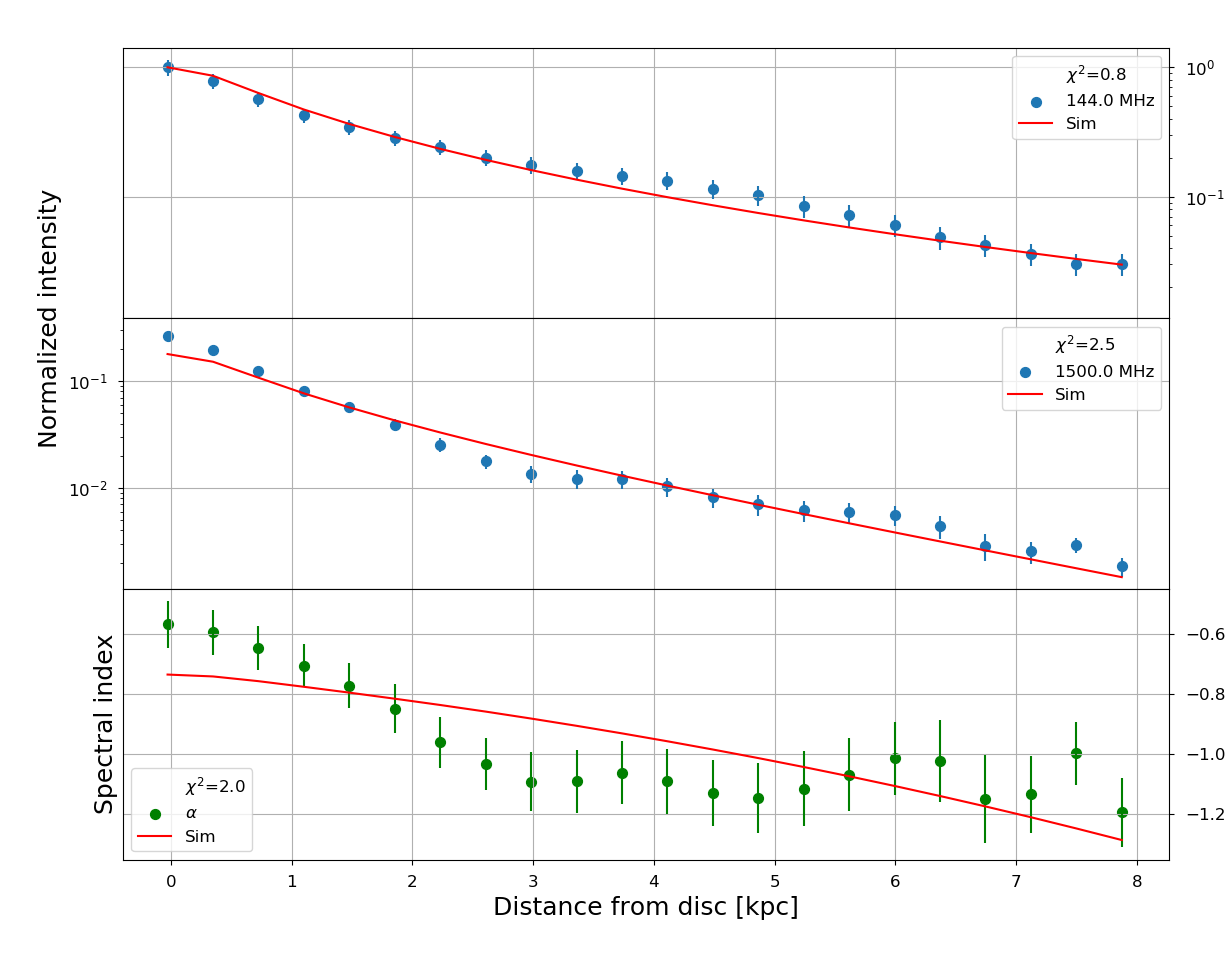}
\end{subfigure}
\\
\begin{subfigure}{0.49\linewidth}
\centering
\includegraphics[width=1\linewidth]{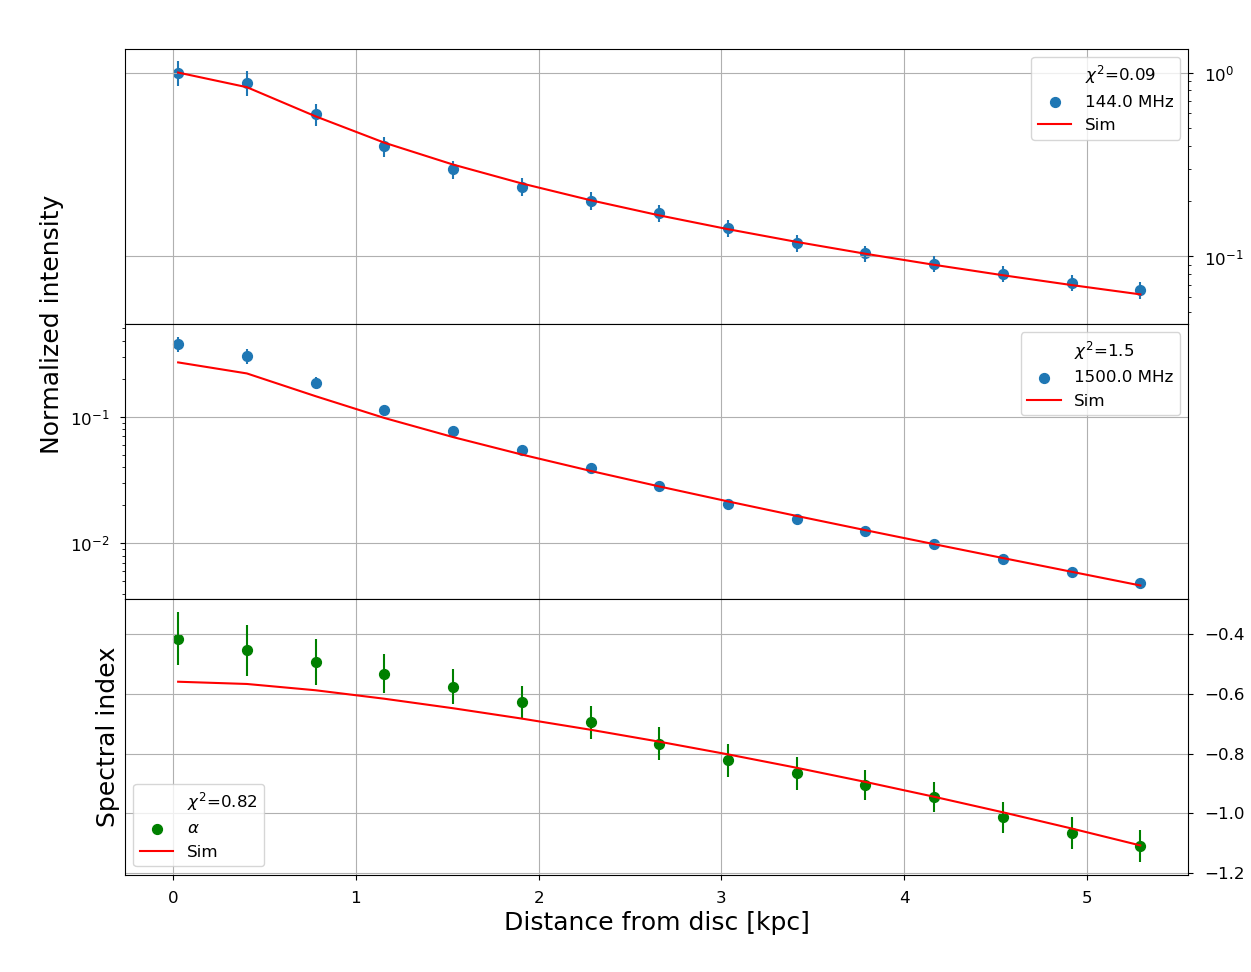}
\end{subfigure}
\hfill
\begin{subfigure}{0.49\linewidth}
\centering
\includegraphics[width=1\linewidth]{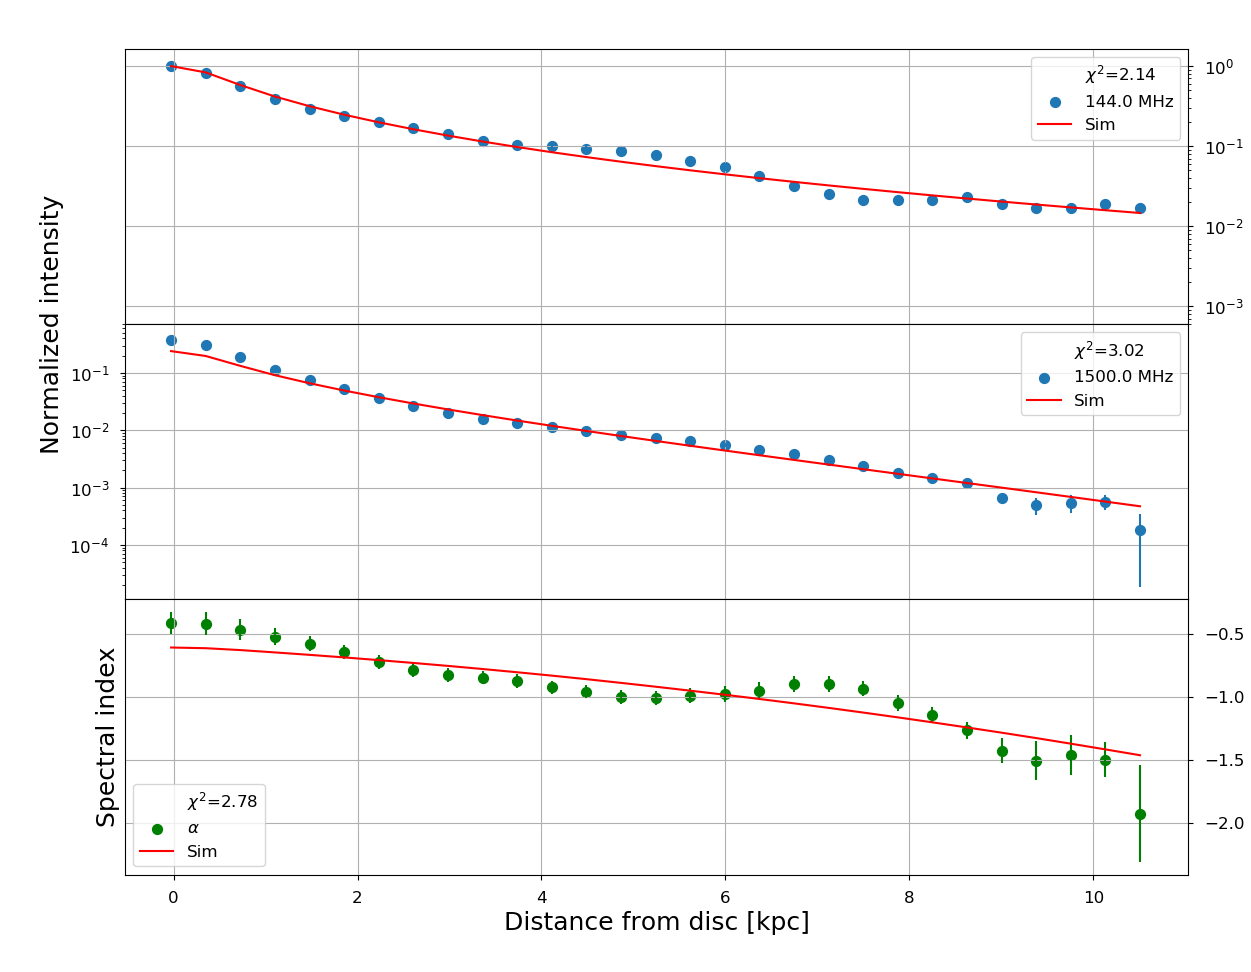}
\end{subfigure}
\\
\begin{subfigure}{0.49\linewidth}
\centering
\includegraphics[width=1\linewidth]{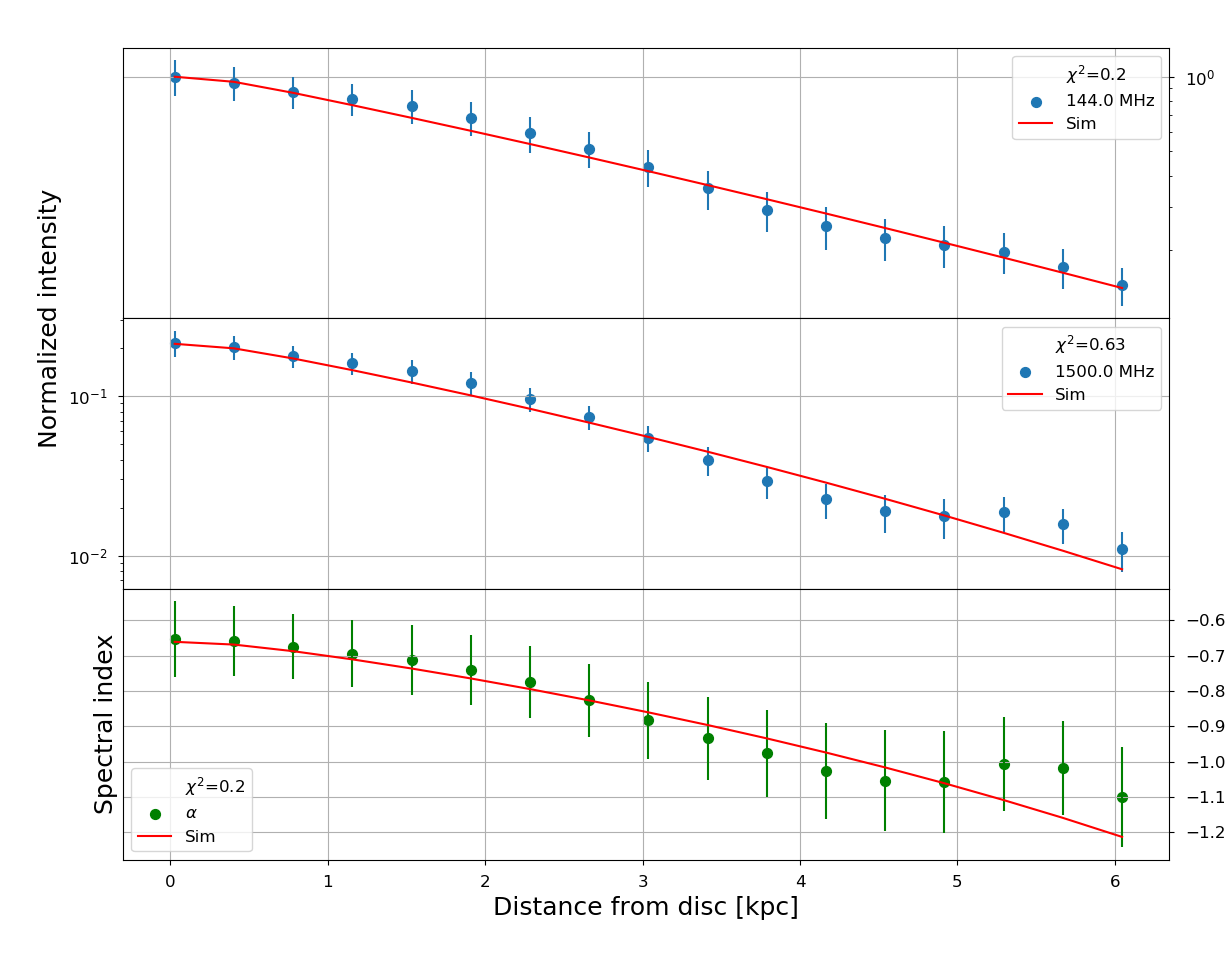}
\end{subfigure}
\hfill
\begin{subfigure}{0.49\linewidth}
\centering
\includegraphics[width=1\linewidth]{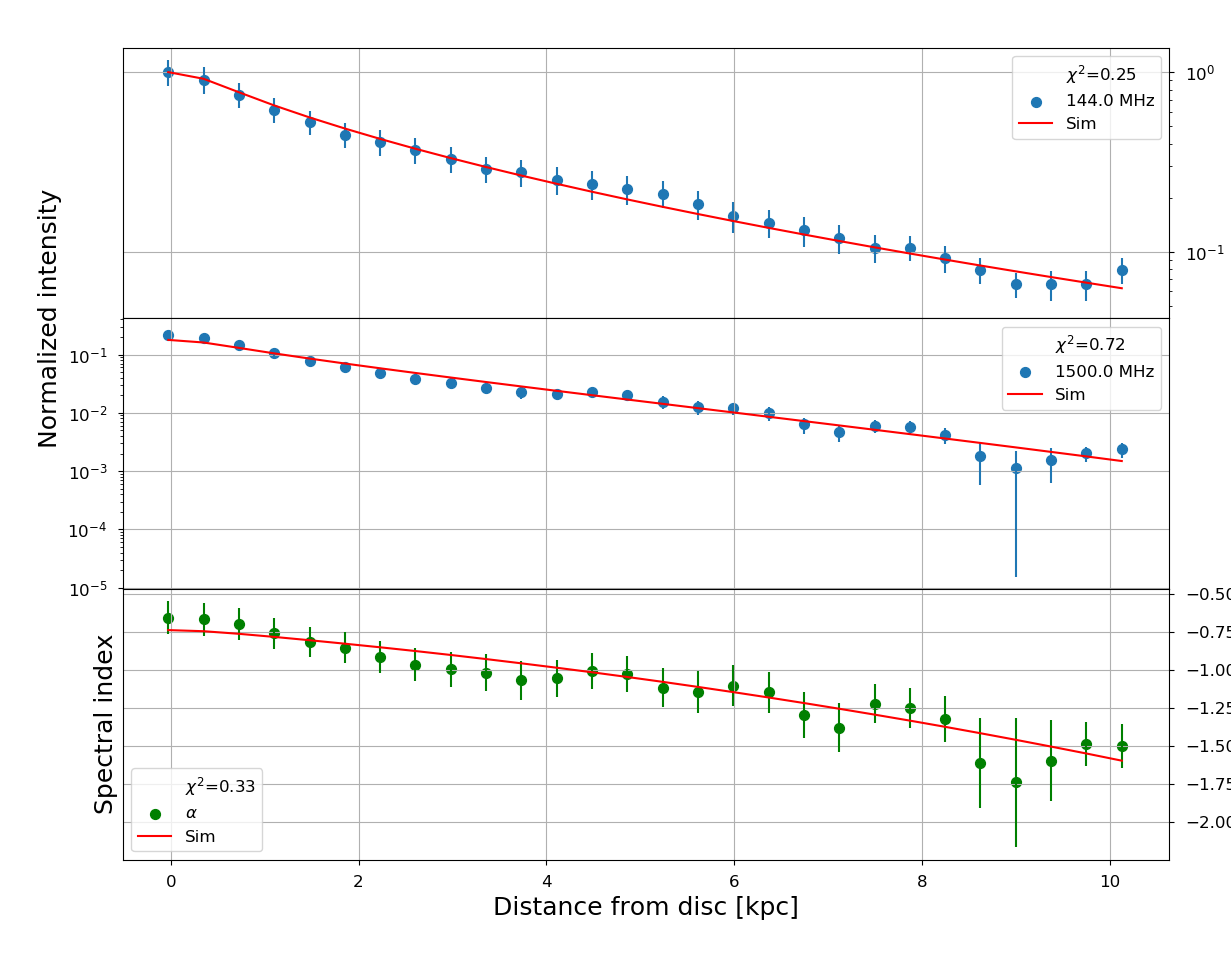}
\end{subfigure}
\caption{\texttt{SPINNAKER} profiles of NGC~4631 (all advection). Strips are presented as follows: top left: LR, top right: UR, middle left: LM, middle right: UM, bottom left: LL, and bottom right: UL.}
\end{figure*}
